# Supplementary material for: A Cubic Regularization Approach for Finding Local Minimax Points in Nonconvex Minimax Optimization
Source: arXiv:2110.07098 source file (2023-02-19)
Supplement: Supplementary file 1 [file supplementary.tex]

\clearpage
\appendix{
{\centering\Large \textbf{Supplementary Materials}}

The proof of \Cref{coro: mu} is based on the results in other theorems. Thus, we postpone its proof to the end of the supplementary material.

\section*{Proof of \Cref{thm: 2}}

\thmfunc*
\begin{proof}
	We first recall the following fundamental result proved in \cite{Nesterov2006}, which serves as a convenient reference.
	\begin{thm}[Theorem 2, \cite{Nesterov2006}]\label{thm: 1}
		Let \Cref{assum: f} hold. Then, the sequence $\{\xb_{k}\}_k$ generated by CR satisfies 
		\begin{enumerate}[leftmargin=*,topsep=0pt,noitemsep]
			\item The set of limit points $\omega(\xb_{0})$ of $\{\xb_k\}_k$ is nonempty and compact, all of which are second-order stationary points;
			\item The sequence $\{f(\xb_{k}) \}_k$ decreases to a finite limit $\bar{f}$, which is the constant function value evaluated on the set $\omega(\xb_{0})$. 
		\end{enumerate}
	\end{thm}
	
	From the results of \Cref{thm: 1} we conclude that $\dist_{\omega(\xb_{0})}(\xb_{k}) \to 0$, $f(\xb_{k}) \downarrow \bar{f}$ and $\omega(\xb_{0})$ is a compact set on which the function value is the constant $\bar{f}$. Then, it is clear that for any fixed $\epsilon>0, \lambda>0$ and all $k\ge k_0$ with $k_0$ being sufficiently large, $\xb_k \in \{\xb: \dist_{\omega(\xb_{0})}(\xb)<\varepsilon, \bar{f} < f(\xb) <\bar{f} + \lambda\}$. Hence, all the conditions of the \KL property in \Cref{def: KL} are satisfied, and we can exploit the \KL inequality in \cref{eq: KL}. 
	
	Denote $r_k := f(\xb_{k}) - \bar{f}$. For all $k\ge k_0$ we obtain that 
	\begin{align}
	r_k \overset{(i)}{\le} C \|\nabla f(\xb_{k})\|^{\frac{1}{1-\theta}} \overset{(ii)}{\le} C\|\xb_{k} - \xb_{k-1}\|^{\frac{2}{1-\theta}} \overset{(iii)}{\le} C(r_{k-1} - r_{k})^{\frac{2}{3(1-\theta)}}, \label{eq: supp3}
	\end{align}
	where (i) follows from the \KL property in \cref{eq: KLsimple}, (ii) and (iii) follow from the dynamics of CR in \Cref{table: 1} and we have absorbed all constants into $C$. Define $\delta_k = r_k C^{\frac{3(1-\theta)}{3\theta-1}}$, then the above inequality can be rewritten as
	\begin{align}
	\delta_{k-1} - \delta_{k} \ge \delta_k^{\frac{3(1-\theta)}{2}}, \quad \forall k \ge k_0. \label{eq: supp2}
	\end{align}
	Next, we discuss the convergence rate of $\delta_k$ under different regimes of $\theta$. 
	
	\textbf{Case 1: $\theta = 1$.} 
	
	In this case, the \KL property in \cref{eq: KL} satisfies $\varphi'(t) = c$ and implies that $\|\nabla f(\xb_{k})\| \ge \frac{1}{c}$ for some constant $c>0$. On the other hand, by the dynamics of CR in \Cref{table: 1}, we obtain that 
	\begin{align}
	f(\xb_{k+1}) \le f(\xb_{k}) - \frac{M}{12} \|\xb_{k+1} - \xb_{k} \|^3 \le f(\xb_{k}) - \frac{M}{12} (\frac{2}{L+M})^{\frac{3}{2}}\|\nabla f(\xb_{k})\|^{\frac{3}{2}}.
	\end{align}
	Combining these two facts yields the conclusion that for all $k\ge k_0$
	$$f(\xb_{k+1}) \le f(\xb_{k}) - C$$
	for some constant $C>0$. Then, we conclude that $f(\xb_{k}) \downarrow -\infty$, which contradicts the fact that $f(\xb_{k}) \downarrow \bar{f} > -\infty$ (since $f$ is bounded below). Hence, we must have $f(\xb_{k}) \equiv \bar{f}$ for all sufficiently large $k$. 
	
	\textbf{Case 2: $\theta \in (\frac{1}{3}, 1)$.} 
	
	In this case $0< \frac{3(1-\theta)}{2} <1$. Since $\delta_k \to 0$ as $r_k \to 0$, $\delta_k^{\frac{3(1-\theta)}{2}}$ is order-wise larger than $\delta_k$ for all sufficiently large $k$. Hence, for all sufficiently large $k$, \cref{eq: supp2} reduces to
	\begin{align}
	\delta_{k-1} \ge \delta_k^{\frac{3(1-\theta)}{2}}.
	\end{align}
	It follows that $\delta_k\downarrow 0$ super-linearly as $\delta_k \le \delta_{k-1}^{\frac{2}{3(1-\theta)}}$. Since $\delta_k = r_k C^{\frac{2}{1-3\theta}}$, we conclude that $r_k \downarrow 0$ super-linearly as $r_k \le C_1r_{k-1}^{\frac{2}{3(1-\theta)}}$ for some constant $C_1>0$. By letting $k_0$ be sufficiently large so that $r_{k_0}$ is sufficiently small, we obtain that
	\begin{align}
	r_k \le C_1r_{k-1}^{\frac{2}{3(1-\theta)}} \le C_1^{k-k_0} r_{k_0}^{(\frac{2}{3(1-\theta)})^{k-k_0}} = \Theta \Bigg( \exp \bigg(-\bigg(\frac{2}{3(1-\theta)}\bigg)^{k-k_0}\bigg) \Bigg).
	\end{align}
	
	\textbf{Case 3: $\theta = \frac{1}{3}$.} 
	
	In this case $\frac{3(1-\theta)}{2} = 1$, and \cref{eq: supp3} reduces to $r_k \le C (r_{k-1} - r_k)$, i.e., $r_k \downarrow 0$ linearly as $r_k \le \frac{C}{1+C} r_{k-1}$ for some constant $C>0$. Thus, we obtain that for all $k \ge k_0$
	\begin{align}
	r_k \le \bigg(\frac{C}{1+C}\bigg)^{k-k_0} r_{k_0} = \Theta \Big( \exp \big(-(k-k_0)\big) \Big).
	\end{align}
	
	\textbf{Case 4: $\theta \in (0, \frac{1}{3})$.} 
	
	In this case, $1< \frac{3(1-\theta)}{2} <\frac{3}{2}$ and $-\frac{1}{2} < \frac{3\theta-1}{2} < 0$. Since $\delta_k\downarrow 0$, we conclude that for all $k\ge k_0$
	\begin{align}
	\delta_{k-1}^{-\frac{3(1-\theta)}{2}} < \delta_{k}^{-\frac{3(1-\theta)}{2}}, \quad\delta_{k-1}^{\frac{3\theta-1}{2}} < \delta_{k}^{\frac{3\theta-1}{2}}.
	\end{align}
	Define an auxiliary function $\phi(t):= \frac{2}{1-3\theta} t^{\frac{3\theta-1}{2}}$ so that $\phi'(t) = -t^{\frac{3(\theta-1)}{2}}$. We next consider two cases. First, suppose that $\delta_k^{\frac{3(\theta-1)}{2}} \le 2 \delta_{k-1}^{\frac{3(\theta-1)}{2}}$. Then for all $k\ge k_0$
	\begin{align}
	\phi(\delta_k) - \phi(\delta_{k-1}) &= \int_{\delta_{k-1}}^{\delta_{k}} \phi'(t) dt =  \int_{\delta_{k}}^{\delta_{k-1}} t^{\frac{3(\theta-1)}{2}} dt \ge (\delta_{k-1} - \delta_{k}) \delta_{k-1}^{\frac{3(\theta-1)}{2}} \\
	&\overset{(i)}{\ge} \frac{1}{2}(\delta_{k-1} - \delta_{k}) \delta_{k}^{\frac{3(\theta-1)}{2}} \overset{(ii)}{\ge} \frac{1}{2},
	\end{align}
	where (i) utilizes the assumption and (ii) uses \cref{eq: supp2}. 
	
	Second, suppose that $\delta_k^{\frac{3(\theta-1)}{2}} \ge 2 \delta_{k-1}^{\frac{3(\theta-1)}{2}}$. Then $\delta_{k}^{\frac{3\theta - 1}{2}} \ge 2^{\frac{3\theta - 1}{3(\theta - 1)}} \delta_{k-1}^{\frac{3\theta - 1}{2}}$, which further leads to
	\begin{align}
	\phi(\delta_{k}) - \phi(\delta_{k-1}) &= \frac{2}{1-3\theta} (\delta_{k}^{\frac{3\theta - 1}{2}} - \delta_{k-1}^{\frac{3\theta - 1}{2}}) \ge \frac{2}{1-3\theta} (2^{\frac{3\theta - 1}{3(\theta - 1)}} - 1) \delta_{k-1}^{\frac{3\theta - 1}{2}} \\
	&\ge \frac{2}{1-3\theta} (2^{\frac{3\theta - 1}{3(\theta - 1)}} - 1) \delta_{k_0}^{\frac{3\theta - 1}{2}}.
	\end{align}
	Combining the above two cases and defining $C := \min \{\frac{1}{2}, \frac{2}{1-3\theta} (2^{\frac{3\theta - 1}{3(\theta - 1)}} - 1) \delta_{k_0}^{\frac{3\theta - 1}{2}} \}$, we conclude that for all $k\ge k_0$
	\begin{align}
	\phi(\delta_{k}) - \phi(\delta_{k-1}) \ge C,
	\end{align}
	which further implies that
	\begin{align}
	\phi(\delta_{k}) \ge \sum_{i=k_0 + 1}^{k} \phi(\delta_{i}) - \phi(\delta_{i-1}) \ge C(k-k_0).
	\end{align}
	Substituting the form of $\phi$ into the above inequality and simplifying the expression yields $\delta_{k} \le (\frac{2}{C(1-3\theta)(k-k_0)})^{\frac{2}{1-3\theta}}$. It follows that $r_k \le (\frac{C_3}{k-k_0})^{\frac{2}{1-3\theta}}$ for some $C_3>0$.
	
\end{proof}

\section*{Proof of \Cref{thm: finite length}}
\thmfinitelen*
\begin{proof}
	Recall the definition that $r_k:= f(\xb_k) - \bar{f}$, where $\bar{f}$ is the finite limit of $\{f(\xb_{k}) \}_k$. Also, recall that $k_0\in \mathds{N}$ is a sufficiently large integer. Then, for all $k\ge k_0$, the \KL property implies that
	\begin{align}
	\varphi' (r_k) \ge \frac{1}{\|\nabla f(\xb_k)\|} \ge \frac{2}{(L+M)\|\xb_{k} - \xb_{k-1}\|^2}, \label{eq: supp4}
	\end{align}
	where the last inequality uses the dynamics of CR in \Cref{table: 1}. Note that $\varphi(t) = \frac{c}{\theta} t^{\theta}$ is concave for $\theta \in (0,1]$. Then, by concavity we obtain that 
	\begin{align}
	\varphi(r_k) - \varphi(r_{k+1}) \ge \varphi' (r_k) (r_k - r_{k+1}) \ge \frac{M}{6(L+M)}\frac{\|\xb_{k+1} - \xb_{k}\|^3}{\|\xb_{k} - \xb_{k-1}\|^2}, \label{eq: 7}
	\end{align}
	where the last inequality uses \cref{eq: supp4} and the dynamics of CR in \Cref{table: 1}. 
	Rearranging the above inequality, taking cubic root and summing over $k= k_0,\ldots, n$ yield that (all constants are absorbed in $C$)
	\begin{align}
	\sum_{k=k_0}^{n} \|\xb_{k+1} - \xb_{k}\| &\le C \sum_{k=k_0}^{n} (\varphi(r_k) - \varphi(r_{k+1}))^{\frac{1}{3}} \|\xb_k - \xb_{k-1}\|^{\frac{2}{3}} \\
	&\overset{(i)}{\le} C \left[\sum_{k=k_0}^{n} (\varphi(r_k) - \varphi(r_{k+1}))\right]^{\frac{1}{3}} \left[\sum_{k=k_0}^{n} \|\xb_k - \xb_{k-1}\|\right]^{\frac{2}{3}}  \\
	&\overset{(ii)}{\le} C \left[\varphi(r_{k_0})\right]^{\frac{1}{3}} \left[\sum_{k=k_0}^{n} \|\xb_{k+1} - \xb_{k}\| + \|\xb_{k_0} -\xb_{k_0-1} \|\right]^{\frac{2}{3}}, \label{eq: 6}
	\end{align}
	where (i) applies the H{\"{o}}lder's inequality and (ii) uses the fact that $\varphi \ge 0$. Clearly, we must have $\lim_{n\to \infty} \sum_{k=k_0}^{n} \|\xb_{k+1} - \xb_{k}\| < +\infty$, because otherwise the above inequality cannot hold for all $n$ sufficiently large. We then conclude that $$\sum_{k=k_0}^{\infty} \|\xb_{k+1} - \xb_{k}\| < +\infty,$$
	 and the desired result follows because $k_0$ is a fixed number.
	
\end{proof}

\section*{Proof of \Cref{thm: converge_ite}}
\thmiterate*

\begin{proof}
	We prove the theorem case by case.
	
	\textbf{Case 1: $\theta = 1$.} 
	
	We have shown in case 1 of \Cref{thm: 2} that $f(\xb_k) \downarrow \bar{f}$ within finite number of iterations, i.e., $f(\xb_{k+1}) - f(\xb_k) = 0$ for all $k\ge k_0$. Based on this observation, the dynamics of CR in \Cref{table: 1} further implies that for all $k\ge k_0$
	\begin{align}
		0 = f(\xb_{k+1}) - f(\xb_{k}) \le -\frac{M}{12} \|\xb_{k+1} - \xb_{k}\|^3 \le 0.
	\end{align}
	Hence, we conclude that $\xb_{k+1} = \xb_{k}$ for all $k\ge k_0$, i.e.,	$\xb_k$ converges within finite number of iterations. Since \Cref{thm: finite length} shows that $\xb_k$ converges to some $\bar{\xb}$, the desired conclusion follows.
	
	\textbf{Case 2: $\theta \in (\frac{1}{3}, 1)$.} 
	
	Denote $\Delta_k := \sum_{i=k}^{\infty} \|\xb_{i+1} - \xb_{i} \|$. Note that \Cref{thm: finite length} shows that $\xb_{k} \to \bar{\xb}$. Thus, we have $\|\xb_k - \bar{\xb}\| \le \Delta_k$. Next, we derive the convergence rate of $\Delta_k$.
	
	By \Cref{thm: finite length}, $\lim_{n\to \infty} \sum_{i=k}^{n} \|\xb_{i+1} - \xb_{i}\|$ exists for all $k$. Then, we can let $n \to \infty$ in \cref{eq: 6} and obtain that for all $k \ge k_0$
	\begin{align}
	\Delta_k \le C[\varphi(r_k)]^{\frac{1}{3}} \Delta_{k-1}^{\frac{2}{3}} \le C r_k^{\frac{\theta}{3}} \Delta_{k-1}^{\frac{2}{3}} \overset{(i)}{\le} C(\Delta_{k-1} - \Delta_k)^{\frac{2\theta}{3(1-\theta)}} \Delta_{k-1}^{\frac{2}{3}} \le C\Delta_{k-1}^{\frac{2\theta}{3(1-\theta)} + \frac{2}{3}},
	\end{align}
	where $C$ denotes a universal constant that may vary from line to line, and (i) uses the \KL property and the dynamics of CR, i.e., $r_k \le C \|\nabla f(\xb_k)\|^{\frac{1}{1-\theta}} \le C \|\xb_k - \xb_{k-1}\|^{\frac{2}{1-\theta}}$. Note that in this case we have $\frac{2\theta}{3(1-\theta)} + \frac{2}{3} > 1$, and hence the above inequality implies that $\Delta_k$ converges to zero super-linearly as
	\begin{align}
		\Delta_k \le C^{k-k_0} \Delta_{k_0}^{(\frac{2\theta}{3(1-\theta)} + \frac{2}{3})^{k-k_0}} = \Theta \Bigg( \exp \bigg(-\bigg(\frac{2\theta}{3(1-\theta)} + \frac{2}{3}\bigg)^{k-k_0}\bigg) \Bigg).
	\end{align}
	 Since $\|\xb_k - \bar{\xb}\| \le \Delta_k$, it follows that $\|\xb_k - \bar{\xb}\|$ converges to zero super-linearly as desired.
	 %(Note that $\Delta_{k_0}$ is sufficiently small, and hence the effect of $C^{k-k_0}$ can be ignored by the super-linear diminishing term $\Delta_{k_0}^{(\frac{2\theta}{3(1-\theta)} + \frac{2}{3})^{k-k_0}}$).

	\textbf{Cases 3 \& 4.}
	
	We first derive another estimate on $\Delta_k$ that generally holds for both cases 3 and 4, and then separately consider cases 3 and 4, respectively. 
	
	Fix $\gamma \in (0,1)$ and consider $k\ge k_0$. Suppose that $\|\xb_{k+1} - \xb_{k}\| \ge \gamma \|\xb_{k} - \xb_{k-1}\|$, then \cref{eq: 7} can be rewritten as 
	\begin{align}
	\|\xb_{k+1} - \xb_{k}\| \le \frac{C}{\gamma^2} (\varphi(r_k) - \varphi(r_{k+1}))
	\end{align}
	for some constant $C>0$.
	Otherwise, we have $\|\xb_{k+1} - \xb_{k}\| \le \gamma \|\xb_{k} - \xb_{k-1}\|$. Combing these two inequalities yields that
	\begin{align}
	\|\xb_{k+1} - \xb_{k}\| \le \gamma \|\xb_{k} - \xb_{k-1}\| + \frac{C}{\gamma^2} (\varphi(r_k) - \varphi(r_{k+1})).
	\end{align}
	Summing the above inequality over $k = k_0,\ldots, n$ yields that
	\begin{align}
	\sum_{k=k_0}^n \|\xb_{k+1} - \xb_{k}\| &\le \gamma \sum_{k=k_0}^n \|\xb_{k} - \xb_{k-1}\| + \frac{C}{\gamma^2} (\varphi(r_{k_0}) - \varphi(r_{n+1})) \\
	&\le \gamma \left[\sum_{k=k_0}^n \|\xb_{k+1} - \xb_{k}\| + \|\xb_{k_0} - \xb_{k_0-1}\|\right] + \frac{C}{\gamma^2}\varphi(r_{k_0}).
	\end{align}
	Rearranging the above inequality yields that
	\begin{align}
	\sum_{k=k_0}^n \|\xb_{k+1} - \xb_{k}\| \le \frac{\gamma}{1 - \gamma} \|\xb_{k_0} - \xb_{k_0-1}\| + \frac{C}{\gamma^2(1 - \gamma)}\varphi(r_{k_0}).
	\end{align}
	Recall $\Delta_k := \sum_{i=k}^{\infty} \|\xb_{i+1} - \xb_{i} \| < + \infty$. Letting $n\to \infty$ in the above inequality yields that for all sufficiently large $k$
	\begin{align}
	\Delta_{k} &\le \frac{\gamma}{1 - \gamma} (\Delta_{k - 1} - \Delta_{k}) + \frac{C}{\gamma^2(1 - \gamma)\theta}r_{k}^\theta \\
	&\overset{(i)}{\le} \frac{\gamma}{1 - \gamma} (\Delta_{k - 1} - \Delta_{k}) + \frac{C}{\gamma^2(1 - \gamma)\theta}\|\xb_{k} - \xb_{k-1}\|^{\frac{2\theta}{1 - \theta}} \\
	&\le \frac{\gamma}{1 - \gamma} (\Delta_{k - 1} - \Delta_{k}) + \frac{C}{\gamma^2(1 - \gamma)\theta}(\Delta_{k - 1} - \Delta_{k})^{\frac{2\theta}{1 - \theta}}, \label{eq: 8}
	\end{align}
	where (i) uses the \KL property and the dynamics of CR, i.e., $r_k \le C \|\nabla f(\xb_k)\|^{\frac{1}{1-\theta}} \le C \|\xb_k - \xb_{k-1}\|^{\frac{2}{1-\theta}}$. 
	
	\textbf{Case 3:} $\theta = \frac{1}{3}$. In this case, $\frac{2\theta}{1 - \theta} = 1$ and \cref{eq: 8} implies that $\Delta_{k} \le C (\Delta_{k - 1} - \Delta_{k})$ for all sufficiently large $k$, i.e., $\Delta_k$ converges to zero linearly as $\Delta_{k} \le (\frac{C}{1+C})^{k-k_0} \Delta_{k_0}$. The desired result follows since $\|\xb_{k} - \bar{\xb}\| \le \Delta_k$.
	
	\textbf{Case 4:} $\theta \in (0, \frac{1}{3})$. In this case, $0<\frac{2\theta}{1 - \theta} < 1$ and \cref{eq: 8} can be asymptotically rewritten as $\Delta_k \le \frac{C}{\gamma^2(1 - \gamma)\theta}(\Delta_{k - 1} - \Delta_{k})^{\frac{2\theta}{1 - \theta}}$. This further implies that
	\begin{align}
	\Delta_k^{\frac{1-\theta}{2\theta}} \le C (\Delta_{k-1} - \Delta_k)
	\end{align}
	for some constant $C>0$.
	Define $h(t) = t^{-\frac{1-\theta}{2\theta}}$ and fix $\beta > 1$. Suppose first that $h(\Delta_k) \le \beta h(\Delta_{k-1})$. Then the above inequality implies that
	\begin{align}
	1 &\le C \frac{\Delta_{k-1} - \Delta_k}{\Delta_k^{\frac{1-\theta}{2\theta}}} = C(\Delta_{k-1} - \Delta_k) h(\Delta_k) \le C\beta(\Delta_{k-1} - \Delta_k) h(\Delta_{k-1}) \\
	&\le C\beta \int_{\Delta_k}^{\Delta_{k-1}} h(t) dt = C\beta \frac{2\theta}{3\theta -1} (\Delta_{k-1}^{\frac{3\theta-1}{2\theta}} - \Delta_{k}^{\frac{3\theta-1}{2\theta}}).
	\end{align}
	Set $\mu:= \frac{1-3\theta}{2C\beta \theta} > 0, \nu := \frac{3\theta - 1}{2\theta} < 0$. Then the above inequality can be rewritten as
	\begin{align}
	\Delta_k^\nu - \Delta_{k-1}^\nu \ge \mu.
	\end{align}
	Now suppose $h(\Delta_k) > \beta h(\Delta_{k-1})$, which implies that $\Delta_{k} < q\Delta_{k-1}$ with $q = \beta^{-\frac{2\theta}{1-\theta}} \in (0,1)$. Then, we conclude that $\Delta_k^\nu \ge q^\nu \Delta_{k-1}^\nu$ and hence $\Delta_k^\nu - \Delta_{k-1}^\nu \ge (q^\nu - 1) \Delta_{k-1}^\nu$. Since $q^\nu - 1 > 0$ and $\Delta_{k-1}^\nu \to +\infty$, there must exist $\bar{\mu}>0$ such that $(q^\nu - 1) \Delta_{k-1}^\nu \ge \bar{\mu}$ for all sufficiently large $k$. Thus, we conclude that $\Delta_k^\nu - \Delta_{k-1}^\nu \ge \bar{\mu}$. Combining two cases, we obtain that for all sufficiently large $k$,
	\begin{align}
	\Delta_k^\nu - \Delta_{k-1}^\nu \ge \min \{\mu, \bar{\mu}\}.
	\end{align}
	Telescoping the above inequality over $k = k_0, \ldots, k$ yields that 
	\begin{align}
	\Delta_k \le [\Delta_{k_0}^\nu + \min \{\mu, \bar{\mu}\} (k-k_0)]^{\frac{1}{\nu}} \le \bigg(\frac{C}{k-k_0}\bigg)^{\frac{2\theta}{1-3\theta}},
	\end{align}
	where $C$ is a certain positive constant.
	The desired result then follows from the fact that $ \|\xb_{k} - \bar{\xb}\| \le \Delta_k$.
\end{proof}

\section*{Proof of \Cref{prop: 1}}
\propeb*

\begin{proof}
	The proof idea follows from that in \cite{Yue2018}.	
	Consider any $\xb\in \Omega^c \cap \{\xb\in \RR^d : \dist_\Omega(\xb)<\varepsilon, f_\Omega < f(\xb) <f_\Omega + \lambda\}$, and consider the following differential equation
	\begin{align}\label{eq: 1}
	\ub(0) = \xb, \quad \overset{\bigcdot}{\ub}(t) = -\nabla f(\ub(t)), \quad \forall t>0.
	\end{align}
	As $\nabla f$ is continuously differentiable, it is Lipschitz on every compact set. Thus, by the Picard-Lindel\"{o}f theorem \cite[Theorem II.1.1]{Hartman}, there exists $\nu > 0$ such that \cref{eq: 1} has a unique solution $\ub_\xb (t)$ over the interval $[0, \nu]$. Define $\Delta(t):= f(\ub_\xb (t)) - f_\Omega$. 
	Note that $\Delta(t)>0$ for $t\in [0,\nu]$, as otherwise there exists $\hat{t} \in [0, \nu]$ such that $\ub_\xb (\hat{t}) \in \Omega$ and hence $\ub_\xb \equiv \ub_\xb (\hat{t}) \in \Omega$ is the unique solution to \cref{eq: 1}. This contradicts the fact that $\ub(0) \in \Omega^c$. 
	
	Using \cref{eq: 1} and the chain rule, we obtain that for all $t\in [0, \nu]$
	\begin{align}
	\overset{\bigcdot}{\Delta}(t) = \inner{\nabla f(\ub_\xb (t))}{\overset{\bigcdot}{\ub}_\xb(t)} = - \|\nabla f(\ub_\xb (t))\| \|\overset{\bigcdot}{\ub}_\xb(t)\|.
	\end{align} 
	Applying the \KL property in \cref{eq: KLsimple} to the above equation yields that
	\begin{align}\label{eq: 2}
	\overset{\bigcdot}{\Delta}(t) \le - \left( \frac{\Delta(t)}{C}\right)^{1-\theta} \|\overset{\bigcdot}{\ub}_\xb(t)\|,
	\end{align}
	where $C>0$ is a certain universal constant.
	Since $\Delta(t) > 0$, \cref{eq: 2} can be rewritten as
	\begin{align}
	\|\overset{\bigcdot}{\ub}_\xb(t)\| \le -\frac{C^{1-\theta}}{\theta} (\Delta(t)^\theta)'.
	\end{align}
	Based on the above inequality, for any $0\le a<b<\nu$ we obtain that
	\begin{align}
	\|\ub_\xb(b) - \ub_\xb(a)\| &= \|\int_{a}^{b} \overset{\bigcdot}{\ub}_\xb(t) dt\| \le \int_{a}^{b} \|\overset{\bigcdot}{\ub}_\xb(t) \|dt \nonumber\\
	&\le - \int_{a}^{b} \frac{C^{1-\theta}}{\theta} [\Delta(t)^\theta]' dt = \frac{C^{1-\theta}}{\theta} [\Delta(a)^\theta - \Delta(b)^\theta]. \label{eq: 3}
	\end{align}
	In particular, setting $a=0$ in \cref{eq: 3} and noting that $\ub_\xb(0) = \xb$, we further obtain that
	\begin{align}
	\|\ub_\xb(b) - \xb\| \le \frac{C^{1-\theta}}{\theta} (f(\xb) - f_\Omega)^\theta. \label{eq: supp1}
	\end{align}
	
	Next, we show that $\nu = +\infty$. Suppose $\nu < +\infty$, then \cite[Corollary II.3.2]{Hartman} shows that $\|\ub_\xb(t)\| \to +\infty$ as $t \to \nu$. However, 
	\cref{eq: supp1} implies that
	\begin{align*}
	\|\ub_\xb(t)\| \le \|\xb\| + \|\ub_\xb(t) - \xb\| \le \|\xb\| + \frac{C^{1-\theta}}{\theta}(f(\xb) - f_\Omega)^\theta < +\infty,
	\end{align*}
	which leads to a contradiction. Thus, $\nu = +\infty$. 
	
	Since $\overset{\bigcdot}{\Delta}(t) \le 0$, $\Delta(t)$ is non-increasing. Hence, the nonnegative sequence $\{\Delta(t)\}$ has a limit. Then, \cref{eq: 3} further implies that $\{\ub_\xb(t)\}$ is a Cauchy sequence and hence has a limit $\ub_\xb(\infty)$. Suppose $\nabla f(\ub_\xb(\infty)) \ne \zero$. Then we obtain that $\lim_{t \to \infty}\overset{\bigcdot}{\Delta}(t) = - \|\nabla f(\ub_\xb(\infty))\|^2 < 0$, which contradicts the fact that $\lim_{t\to \infty} \Delta(t)$ exists. Thus, $\nabla f(\ub_\xb(\infty)) = \zero$, and this further implies that $\ub_\xb(\infty)\in \Omega, f(\ub_\xb(\infty)) = f_\Omega$ by the \KL property in \cref{eq: KLsimple}. We then conclude that 
	\begin{align}
	\dist_\Omega(\xb) \le \|\xb - \ub_\xb(\infty)\| = \lim_{t \to \infty} \|\xb - \ub_\xb(t)\| \le \frac{C^{1-\theta}}{\theta}(f(\xb) - f_\Omega)^\theta.
	\end{align}
Combining the above inequality with the \KL property in \cref{eq: KLsimple}, we obtain the desired \KL error bound.
\end{proof}

\section*{Proof of \Cref{thm: dist}}
\thmdist*

\begin{proof}
   We prove the theorem case by case.
   
	\textbf{Case 1: $\theta = 1$.} 
	
	We have proved in \Cref{thm: converge_ite} that $\xb_k \to \bar{\xb}\in \Omega$ within finite number of iterations. 
	Since $\dist_\Omega(\xb_k) \le \|\xb_k - \bar{\xb}\|$, we conclude that $\dist_\Omega(\xb_k)$ converges to zero within finite number of iterations. 
	
	\textbf{Case 2: $\theta \in (\frac{1}{3}, 1)$.} 
	
	By the \KL error bound in \Cref{prop: 1}, we obtain that
	\begin{align}
	\dist_\Omega(\xb_{k+1}) \le C \|\nabla f(\xb_{k+1})\|^{\frac{\theta}{1-\theta}} \le C\|\xb_{k+1} - \xb_k\|^{\frac{2\theta}{1-\theta}}, \label{eq: supp5}
	\end{align}
	where the last inequality uses the dynamics of CR in \Cref{table: 1}. On the other hand, \cite[Lemma 1]{Yue2018} shows that 
	\begin{align}
		\|\xb_{k+1} - \xb_k\| \le C \dist_\Omega(\xb_k). \label{eq: supp6}
	\end{align}
  Combining \cref{eq: supp5} and \cref{eq: supp6} yields that
	\begin{align}
	\dist_\Omega(\xb_{k+1}) \le C \dist_\Omega(\xb_{k})^{\frac{2\theta}{1-\theta}}.
	\end{align}
	Note that in this case we have $\frac{2\theta}{1-\theta} > 1$. Thus, $\dist_\Omega(\xb_{k})$ converges to zero super-linearly as desired.
	
	\textbf{Cases 3 \& 4: $\theta \in (0, \frac{1}{3}]$.} 
	
	Note that $\dist_\Omega(\xb_k) \le \|\xb_k - \bar{\xb}\|$. The desired results follow from Cases 3 \& 4 in
	\Cref{thm: converge_ite}.
	
\end{proof}

\section*{Proof of \Cref{coro: mu}}
\thmmu*

\begin{proof}

By the dynamics of CR in \Cref{table: 1}, we obtain that
\begin{align}
\|\nabla f(\xb_{k+1})\| &\le \frac{L+M}{2} \|\xb_{k+1} - \xb_{k}\|^2, \\
-\lambda_{\min} (\nabla^2 f(\xb_{k+1})) &\le \frac{2L + M}{2} \|\xb_{k+1} - \xb_{k}\|.
\end{align}
The above two inequalities imply that $\mu(\xb_{k}) \le \|\xb_{k+1} - \xb_{k}\|$. Also, \cite[Lemma 1]{Yue2018} shows that $\|\xb_{k+1} - \xb_{k}\|\le C \dist_\Omega(\xb_{k})$. Then, the desired convergence result for $\mu(\xb_{k})$ follows from \Cref{thm: dist}.

\end{proof}
