# Supplementary material for: A Cubic Regularization Approach for Finding Local Minimax Points in Nonconvex Minimax Optimization
Source: arXiv:2110.07098 source file (2023-02-19)
Supplement: Supplementary file 3 [file cubic_regularization_minimax_supp.pdf]

544

# Appendix

546

547

## Table of Contents

548

A Supporting Lemmas

14

549

B Proof of Proposition 2

18

550

C Proof of Proposition 3

18

551

D Proof of Theorem 1

19

552

E Proof of Theorem 2

20

553

F Convergence Rate of SGA

23

554

G Compute Jacobian-Vector Product

23

555

556

557

558

## A Supporting Lemmas

559

We first prove the following auxiliary lemma that bounds the spectral norm of the Jacobian matrices.

560

561

**Lemma 2.** *Let Assumption 1 hold. Then, for any  $x \in \mathbb{R}^m$  and  $y \in \mathbb{R}^n$ , the Jacobian matrices of  $f(x, y)$  and  $G(x, y) = [\nabla_{11}f - \nabla_{12}f(\nabla_{22}f)^{-1}\nabla_{21}f](x, y)$  satisfy the following bounds.*

$$\|[\nabla_{22}f(x, y)]^{-1}\| \leq \mu^{-1}, \quad (14)$$

$$\|\nabla_{12}f(x, y)\| = \|\nabla_{21}f(x, y)\| \leq L_1, \quad (15)$$

$$\|\nabla_{11}f(x, y)\| \leq L_1, \quad (16)$$

$$\|G(x, y)\| \leq L_1(1 + \kappa). \quad (17)$$

562

563

The same bounds also hold for  $\widehat{\nabla}_{11}f$ ,  $\widehat{\nabla}_{12}f$ ,  $\widehat{\nabla}_{21}f$ ,  $\widehat{\nabla}_{22}f$  and  $\widehat{G}$  defined in Section 5 under Assumption 2.

*Proof.* We first prove eq. (14). Consider any  $x \in \mathbb{R}^m$  and  $y \in \mathbb{R}^n$ . By Assumption 1 we know that  $f(x, \cdot)$  is  $\mu$ -strongly concave, which implies that  $-\nabla_{22}f(x, y) \succeq \mu I$ . Thus, we further conclude that

$$\|[\nabla_{22}f(x, y)]^{-1}\| = \lambda_{\max}([-\nabla_{22}f(x, y)]^{-1}) = \left(\lambda_{\min}(-\nabla_{22}f(x, y))\right)^{-1} \leq \mu^{-1}.$$

564

Next, we prove eq. (15). Consider any  $x, u \in \mathbb{R}^m$  and  $y \in \mathbb{R}^n$ , we have

$$\begin{aligned} \|\nabla_{21}f(x, y)u\| &= \left\| \frac{\partial}{\partial t} \nabla_2 f(x + tu, y) \Big|_{t=0} \right\| \\ &= \left\| \lim_{t \rightarrow 0} \frac{1}{t} [\nabla_2 f(x + tu, y) - \nabla_2 f(x, y)] \right\| \\ &= \lim_{t \rightarrow 0} \frac{1}{|t|} \|\nabla_2 f(x + tu, y) - \nabla_2 f(x, y)\| \\ &\leq \lim_{t \rightarrow 0} \frac{L_1}{|t|} \|tu\| = L_1 \|u\|, \end{aligned} \quad (18)$$

565

566

567

which implies that  $\|\nabla_{21}f(x, y)\| \leq L_1$ . Since  $f$  is twice differentiable and has continuous second-order derivative, we have  $\nabla_{12}f(x, y)^\top = \nabla_{21}f(x, y)$ , and hence eq. (15) follows. The proof of eq. (16) is similar.

Finally, eq. (17) can be proved as follows using eqs. (14)&(15).

$$\|G(x, y)\| \leq \|\nabla_{11}f(x, y)\| + \|\nabla_{12}f(x, y)\| \|\nabla_{22}f^{-1}(x, y)\| \|\nabla_{21}f(x, y)\| \leq L_1 + L_1\mu^{-1}L_1 = L_1(1 + \kappa).$$

The proof is similar for the stochastic minimax optimization problem (Q) in Section 5 under Assumption 2.  $\square$

The following lemma restates Lemma 3 of [Wang et al., 2018a].

**Lemma 3.** *The solution  $s_{k+1}$  of the cubic regularization problem in Algorithm 1 satisfies the following conditions,*

$$\nabla f(x_t, y_{t+1}) + G(x_t, y_{t+1})s_{t+1} + \frac{1}{2\eta_x}\|s_{t+1}\|s_{t+1} = \mathbf{0}, \quad (19)$$

$$G(x_t, y_{t+1}) + \frac{1}{2\eta_x}\|s_{t+1}\|I \succeq \mathbf{O}, \quad (20)$$

$$\nabla f(x_t, y_{t+1})^\top s_{t+1} + \frac{1}{2}s_{t+1}^\top G(x_t, y_{t+1})s_{t+1} \leq -\frac{1}{4\eta_x}\|s_{t+1}\|^3. \quad (21)$$

**Lemma 4.** *Suppose the gradient  $\nabla_1 f(x_t, y_{t+1})$  and Hessian  $G(x_t, y_{t+1})$  involved in the cubic-regularization step in Algorithm 1 satisfy the following bounds for all  $t \leq T' - 1$  with  $T' = \min\{t \geq 0 : \|s_{t-1}\| \vee \|s_t\| \leq \epsilon'\}$ :*

$$\|\nabla\Phi(x_t) - \nabla_1 f(x_t, y_{t+1})\| \leq \beta(\|s_t\|^2 + \epsilon'^2), \quad (22)$$

$$\|\nabla^2\Phi(x_t) - G(x_t, y_{t+1})\| \leq \alpha(\|s_t\| + \epsilon'). \quad (23)$$

Then, choosing  $\eta_x \leq (9L_\Phi + 18\alpha + 28\beta)^{-1}$ , the sequence  $\{x_t\}_t$  generated by Algorithm 1 satisfies that for all  $t \leq T' - 2$ ,

$$H_{t+1} - H_t \leq -(L_\Phi + \alpha + \beta)(\|s_{t+1}\|^3 + \|s_t\|^3), \quad (24)$$

where  $H_t = \Phi(x_t) + (L_\Phi + 2\alpha + 3\beta)\|x_t - x_{t-1}\|^3$ . The same conclusion holds for Algorithm 2 by replacing  $\nabla_1 f(x_t, y_{t+1})$ ,  $G(x_t, y_{t+1})$  with their stochastic estimators  $\widehat{\nabla}_1 f(x_t, y_{t+1})$ ,  $\widehat{G}(x_t, y_{t+1})$  respectively.

*Proof.* The proof logic follows that of the proof of Theorem 1 in [Wang et al., 2019]. By the Lipschitz continuity of the Hessian of  $\Phi$ , we obtain that

$$\begin{aligned} & \Phi(x_{t+1}) - \Phi(x_t) \\ & \leq \nabla\Phi(x_t)^\top (x_{t+1} - x_t) + \frac{1}{2}(x_{t+1} - x_t)^\top \nabla^2\Phi(x_t)(x_{t+1} - x_t) + \frac{L_\Phi}{6}\|x_{t+1} - x_t\|^3 \\ & = \nabla_1 f(x_t, y_{t+1})^\top s_{t+1} + \frac{1}{2}s_{t+1}^\top G(x_t, y_{t+1})s_{t+1} + \frac{L_\Phi}{6}\|s_{t+1}\|^3 \\ & \quad + (\nabla\Phi(x_t) - \nabla_1 f(x_t, y_{t+1}))^\top s_{t+1} + \frac{1}{2}s_{t+1}^\top (\nabla^2\Phi(x_t) - G(x_t, y_{t+1}))s_{t+1} \\ & \stackrel{(i)}{\leq} \left(\frac{L_\Phi}{6} - \frac{1}{4\eta_x}\right)\|s_{t+1}\|^3 + \beta\|s_{t+1}\|(\|s_t\|^2 + \epsilon'^2) + \frac{\alpha}{2}\|s_{t+1}\|^2(\|s_t\| + \epsilon') \\ & \stackrel{(ii)}{\leq} \left(\frac{L_\Phi}{6} - \frac{1}{4\eta_x}\right)\|s_{t+1}\|^3 + \left(\frac{\alpha}{2} + \beta\right)(2\|s_{t+1}\|^3 + \|s_t\|^3 + \epsilon'^3) \\ & \stackrel{(iii)}{\leq} \left(\frac{L_\Phi}{6} - \frac{1}{4\eta_x}\right)\|s_{t+1}\|^3 + \left(\frac{\alpha}{2} + \beta\right)(3\|s_{t+1}\|^3 + 2\|s_t\|^3) \\ & \leq -\left(\frac{1}{4\eta_x} - \frac{L_\Phi}{6} - \frac{3\alpha}{2} - 3\beta\right)\|s_{t+1}\|^3 + (\alpha + 2\beta)\|s_t\|^3, \\ & \stackrel{(iv)}{\leq} -(2L_\Phi + 3\alpha + 4\beta)\|s_{t+1}\|^3 + (\alpha + 2\beta)\|s_t\|^3 \end{aligned}$$

where (i) uses eqs. (21), (22)& (23), (ii) uses the inequality that  $ab^2 \leq a^3 \vee b^3 \leq a^3 + b^3, \forall a, b \geq 0$ , (iii) uses  $\epsilon'^3 \leq \|s_t\|^3 \vee \|s_{t+1}\|^3 \leq \|s_t\|^3 + \|s_{t+1}\|^3, \forall 0 \leq t \leq T' - 2$  based on the termination

586 criterion of  $T'$ , and (iv) uses  $\eta_x \leq (9L_\Phi + 18\alpha + 28\beta)^{-1}$ . Eq. (24) follows from the above inequality  
 587 by defining  $H_t = \Phi(x_t) + (L_\Phi + 2\alpha + 3\beta)\|x_t - x_{t-1}\|^2$ .

588 Note that the cubic-regularization step in Algorithm 2 simply replaces  $\nabla_1 f(x_t, y_{t+1})$ ,  $G(x_t, y_{t+1})$   
 589 in Algorithm 1 with their stochastic estimators  $\hat{\nabla}_1 f(x_t, y_{t+1})$ ,  $\hat{G}(x_t, y_{t+1})$  respectively. Hence, eq.  
 590 (24) holds for Algorithm 2 after such replacement in eqs. (22) & (23).  $\square$

591 **Lemma 5.** Suppose all the conditions of Lemma 4 hold. If  $T \geq \frac{\Phi(x_0) - \Phi^* + (L_\Phi + 3\alpha + 4\beta)\epsilon'^2}{(L_\Phi + \alpha + \beta)\epsilon'^3}$  in  
 592 Algorithm 1, then  $T' = \min\{t \geq 1 : \|s_{t-1}\| \vee \|s_t\| \leq \epsilon'\} \leq \frac{\Phi(x_0) - \Phi^* + (L_\Phi + 3\alpha + 4\beta)\epsilon'^2}{(L_\Phi + \alpha + \beta)\epsilon'^3} \leq T$ .  
 593 Consequently, the output of Algorithm 1 has the following convergence rate

$$\|\nabla\Phi(x_{T'})\| \leq \left(\frac{1}{2\eta_x} + L_\Phi + 2\alpha + 2\beta\right)\epsilon'^2, \quad (25)$$

$$\nabla^2\Phi(x_{T'}) \succeq -\left(\frac{1}{2\eta_x} + L_\Phi + 2\alpha\right)\epsilon'I. \quad (26)$$

594 The same conclusion holds for Algorithm 2 by replacing  $\nabla_1 f(x_t, y_{t+1})$ ,  $G(x_t, y_{t+1})$  in the conditions  
 595 (22) & (23) with their stochastic estimators  $\hat{\nabla}_1 f(x_t, y_{t+1})$ ,  $\hat{G}(x_t, y_{t+1})$  respectively.

596 *Proof.* The proof logic follows that of the proof of Theorem 1 in [Wang et al., 2019].

597 Suppose  $T' \leq T$  does not hold, i.e.,  $\|s_{t-1}\| \vee \|s_t\| > \epsilon', \forall 1 \leq t \leq T$ , which implies that eq. (24)  
 598 holds for all  $0 \leq t \leq T - 1$  based on Lemma 4.

599 On one hand, telescoping eq. (24) over  $t = 0, 1, \dots, T - 1$  yield that

$$\begin{aligned} H_0 - H_T &\geq (L_\Phi + \alpha + \beta) \sum_{t=0}^{T-1} (\|s_{t+1}\|^3 + \|s_t\|^3) \\ &\geq (L_\Phi + \alpha + \beta) \sum_{t=0}^{T-1} (\|s_t\| \vee \|s_{t+1}\|)^3 \\ &> T(L_\Phi + \alpha + \beta)\epsilon'^3 \\ &\geq \Phi(x_0) - \Phi^* + (L_\Phi + 3\alpha + 4\beta)\epsilon'^2. \end{aligned} \quad (27)$$

600 On the other hand, recalling the definition of  $H_t$  in Lemma 4, we have

$$\begin{aligned} H_0 - H_T &= \Phi(x_0) - \Phi(x_T) + (L_\Phi + 2\alpha + 3\beta)(\|s_0\|^2 - \|s_T\|^2) \\ &\stackrel{(i)}{\leq} \Phi(x_0) - \Phi^* + (L_\Phi + 3\alpha + 4\beta)\epsilon'^2, \end{aligned} \quad (28)$$

601 where (i) uses  $\|s_0\| = \epsilon'$  and  $\Phi(x_T) \geq \Phi^* = \min_{x \in \mathbb{R}^m} \Phi(x)$ . Note that eqs. (27) & (28) contradict.

602 Therefore, we must have  $1 \leq T' \leq T$  for any  $T \geq \frac{\Phi(x_0) - \Phi^* + (L_\Phi + 3\alpha + 4\beta)\epsilon'^2}{(L_\Phi + \alpha + \beta)\epsilon'^3}$ , which implies that

603  $T' \leq \frac{\Phi(x_0) - \Phi^* + (L_\Phi + 3\alpha + 4\beta)\epsilon'^2}{(L_\Phi + \alpha + \beta)\epsilon'^3} \leq T$ .

604 Finally, we conclude that

$$\begin{aligned} &\|\nabla\Phi(x_{T'})\| \\ &\stackrel{(i)}{=} \left\| \nabla\Phi(x_{T'}) - \nabla f(x_{T'-1}, y_{T'}) - G(x_{T'-1}, y_{T'})_{s_{T'}} - \frac{1}{2\eta_x} \|s_{T'}\| s_{T'} \right\| \\ &\leq \|\nabla\Phi(x_{T'}) - \nabla\Phi(x_{T'-1}) - \nabla^2\Phi(x_{T'-1})_{s_{T'}}\| + \|\nabla\Phi(x_{T'-1}) - \nabla f(x_{T'-1}, y_{T'})\| \\ &\quad + \|\nabla^2\Phi(x_{T'-1})_{s_{T'}} - G(x_{T'-1}, y_{T'})_{s_{T'}}\| + \frac{1}{2\eta_x} \|s_{T'}\|^2 \\ &\stackrel{(ii)}{\leq} \left(L_\Phi + \frac{1}{2\eta_x}\right) \|s_{T'}\|^2 + \beta(\|s_{T'-1}\|^2 + \epsilon'^2) + \alpha(\|s_{T'-1}\| + \epsilon') \|s_{T'}\| \\ &\stackrel{(iii)}{\leq} \left(\frac{1}{2\eta_x} + L_\Phi + 2\alpha + 2\beta\right) \epsilon'^2, \end{aligned} \quad (29)$$

where (i) uses eq. (19), (ii) uses eqs. (22) & (23) and the item 2 of Proposition 2 that  $\nabla^2\Phi$  is  $L_\Phi$ -Lipschitz, and (iii) uses  $\|s_{T'-1}\| \vee \|s_{T'}\| \leq \epsilon'$ . Also,

$$\begin{aligned}
\nabla^2\Phi(x_{T'}) &\stackrel{(i)}{\succeq} G(x_{T'-1}, y_{T'}) - \|G(x_{T'-1}, y_{T'}) - \nabla^2\Phi(x_{T'})\|I \\
&\stackrel{(ii)}{\succeq} -\frac{1}{2\eta_x}\|s_{T'}\|I - \|G(x_{T'-1}, y_{T'}) - \nabla^2\Phi(x_{T'-1})\|I - \|\nabla^2\Phi(x_{T'}) - \nabla^2\Phi(x_{T'-1})\|I \\
&\stackrel{(iii)}{\succeq} -\left(\frac{1}{2\eta_x} + L_\Phi\right)\|s_{T'}\|I - \alpha(\|s_{T'-1}\| + \epsilon')I \\
&\stackrel{(iv)}{\succeq} -\left(\frac{1}{2\eta_x} + L_\Phi + 2\alpha\right)\epsilon'I,
\end{aligned} \tag{30}$$

where (i) uses Weyl's inequality, (ii) uses eq. (20), (iii) uses eq. (23) and the item 2 of Proposition 2 that  $\nabla^2\Phi$  is  $L_\Phi$ -Lipschitz, and (iv) uses  $\|s_{T'-1}\| \vee \|s_{T'}\| \leq \epsilon'$ .  $\square$

For the stochastic minimax optimization problem (Q) in Section 5, we prove the following supporting lemma on the error of the stochastic estimators.

**Lemma 1.** Fix any  $0 < \epsilon_1 \leq 2L_0$ ,  $0 < \epsilon_2 \leq 4L_1$  and choose the following batch sizes

$$|B_1| \geq \mathcal{O}\left(\frac{L_0^2}{\epsilon_1^2} \ln \frac{m}{\delta}\right), \tag{8}$$

$$|B_{11}|, |B_{12}|, |B_{21}|, |B_{22}| \geq \mathcal{O}\left(\frac{L_1^2}{\epsilon_2^2} \ln \frac{m+n}{\delta}\right). \tag{9}$$

Then, the stochastic approximators satisfy the following error bounds with probability at least  $1 - \delta$ .

$$\|\widehat{\nabla}_1 f(x, y) - \nabla_1 f(x, y)\| \leq \epsilon_1, \tag{10}$$

$$\|\widehat{\nabla}_{k,\ell}^2 f(x, y) - \nabla_{k,\ell}^2 f(x, y)\| \leq \epsilon_2, \forall k, \ell \in \{1, 2\}, \tag{11}$$

$$\|\widehat{G}(x, y) - G(x, y)\| \leq (\kappa + 1)^2 \epsilon_2. \tag{12}$$

*Proof.* Based on Lemmas 6 & 8 in [Kohler and Lucchi, 2017], we obtain that with probability at least  $1 - \delta$ , the following bounds hold. (We replaced  $\delta$  in [Kohler and Lucchi, 2017] with  $\delta/5$  by applying union bound to the following 5 events.)

$$\|\widehat{\nabla}_1 f(x, y) - \nabla_1 f(x, y)\| \leq 4\sqrt{2}L_0 \sqrt{\frac{\ln(10m/\delta) + 1/4}{|B_1|}} \leq \epsilon_1, \tag{31}$$

$$\|\widehat{\nabla}_{k,\ell}^2 f(x, y) - \nabla_{k,\ell}^2 f(x, y)\| \leq 4L_1 \sqrt{\frac{\ln(10(m \vee n)/\delta)}{|B_{k,\ell}|}} \leq \epsilon_2; k, \ell \in \{1, 2\}. \tag{32}$$

Note that here we only consider the cases that  $|B_1|, |B_{k,\ell}| < N$  for all  $k, \ell \in \{1, 2\}$ . Otherwise,  $|B_1| = N$  yields  $\|\widehat{\nabla}_1 f(x, y) - \nabla_1 f(x, y)\| = 0 < \epsilon_1$  and  $|B_{k,\ell}| = N$  yields  $\|\widehat{\nabla}_{k,\ell}^2 f(x, y) - \nabla_{k,\ell}^2 f(x, y)\| = 0 < \epsilon_2$ . Hence, in both cases, the above high probability bounds hold, which further implies eq. (12) following the argument below.

$$\begin{aligned}
&\|\widehat{G}(x, y) - G(x, y)\| \\
&\leq \|\widehat{\nabla}_{11} f(x, y) - \nabla_{11} f(x, y)\| + \|(\widehat{\nabla}_{12} f(\widehat{\nabla}_{22} f)^{-1} \widehat{\nabla}_{21} f)(x, y) - (\nabla_{12} f(\nabla_{22} f)^{-1} \nabla_{21} f)(x, y)\| \\
&\leq \epsilon_2 + \|(\widehat{\nabla}_{12} f - \nabla_{12} f)(\widehat{\nabla}_{22} f)^{-1} \widehat{\nabla}_{21} f(x, y)\| \\
&\quad + \|\nabla_{12} f((\widehat{\nabla}_{22} f)^{-1} - (\nabla_{22} f)^{-1}) \widehat{\nabla}_{21} f(x, y)\| + \|\nabla_{12} f(\nabla_{22} f)^{-1} (\widehat{\nabla}_{21} f - \nabla_{21} f)(x, y)\| \\
&\stackrel{(i)}{\leq} \epsilon_2 + \epsilon_2 \mu^{-1} L_1 + L_1^2 \|\nabla_{22} f(x, y)^{-1}\| \|(\nabla_{22} f - \widehat{\nabla}_{22} f)(x, y)\| \|\widehat{\nabla}_{22} f(x, y)^{-1}\| + L_1 \mu^{-1} \epsilon_2 \\
&\stackrel{(ii)}{\leq} \epsilon_2 + 2\kappa \epsilon_2 + L_1^2 \mu^{-2} \epsilon_2 \leq (\kappa + 1)^2 \epsilon_2.
\end{aligned} \tag{33}$$

where (i) and (ii) use Lemma 2.  $\square$

Regarding the high-probability convergence rate of the inner stochastic gradient ascent (SGA) in Algorithm 2, the following result is a direct application of Theorem 3.1 in [Harvey et al., 2019].

## B Proof of Proposition 2

**Proposition 2.** *Let Assumption 1 hold. Then, the following statements hold.*

1. Define  $G(x, y) = [\nabla_{11}f - \nabla_{12}f(\nabla_{22}f)^{-1}\nabla_{21}f](x, y)$ . Then,  $G$  is a Lipschitz continuous mapping with constant  $L_G = L_2(1 + \kappa)^2$ ;
2. The Hessian of  $\Phi$  satisfies  $\nabla^2\Phi(x) = G(x, y^*(x))$ , and it is Lipschitz continuous with constant  $L_\Phi = L_G(1 + \kappa) = L_2(1 + \kappa)^3$ .

*Proof.* We first prove the item 1. Consider any  $x, x' \in \mathbb{R}^m$  and  $y, y' \in \mathbb{R}^n$ . For convenience we denote  $z = (x, y)$  and  $z' = (x', y')$ . Then, by Assumption 1 and using the bounds of Lemma 2, we have that

$$\begin{aligned}
& \|G(x', y') - G(x, y)\| \\
& \leq \|\nabla_{11}f(x', y') - \nabla_{11}f(x, y)\| + \|\nabla_{12}f(x', y') - \nabla_{12}f(x, y)\| \|\nabla_{22}f(x', y')\|^{-1} \|\nabla_{21}f(x', y')\| \\
& \quad + \|\nabla_{12}f(x, y)\| \|\nabla_{22}f(x', y')\|^{-1} - \|\nabla_{22}f(x, y)\|^{-1} \|\nabla_{21}f(x', y')\| \\
& \quad + \|\nabla_{12}f(x, y)\| \|\nabla_{22}f(x, y)^{-1}\| \|\nabla_{21}f(x', y') - \nabla_{21}f(x, y)\| \\
& \leq L_2\|z' - z\| + (L_2\|z' - z\|)\mu^{-1}L_1 \\
& \quad + L_1^2\|\nabla_{22}f(x', y')\|^{-1} \|\nabla_{22}f(x, y) - \nabla_{22}f(x', y')\| \|\nabla_{22}f(x, y)\|^{-1} + L_1\mu^{-1}(L_2\|z' - z\|) \\
& \leq L_2(1 + 2\kappa)\|z' - z\| + L_1^2\mu^{-1}(L_2\|z' - z\|)\mu^{-1} \\
& \leq L_2(1 + \kappa)^2\|z' - z\|.
\end{aligned}$$

Next, we prove the item 2. Consider any fixed  $x \in \mathbb{R}^m$ , we know that  $f(x, \cdot)$  achieves its maximum at  $y^*(x)$ , where the gradient vanishes, i.e.,  $\nabla_2 f(x, y^*(x)) = \mathbf{0}$ . Thus, we further obtain that

$$\mathbf{0} = \nabla_x \nabla_2 f(x, y^*(x)) = \nabla_{21}f(x, y^*(x)) + \nabla_{22}f(x, y^*(x))\nabla y^*(x),$$

which implies that

$$\nabla y^*(x) = -[\nabla_{22}f(x, y^*(x))]^{-1}\nabla_{21}f(x, y^*(x)). \quad (34)$$

With the above equation, we take derivative of  $\nabla\Phi(x) = \nabla_1 f(x, y^*(x))$  and obtain that

$$\begin{aligned}
\nabla^2\Phi(x) &= \nabla_{11}f(x, y^*(x)) + \nabla_{12}f(x, y^*(x))\nabla y^*(x) \\
&= \nabla_{11}f(x, y^*(x)) - \nabla_{12}f(x, y^*(x))[\nabla_{22}f(x, y^*(x))]^{-1}\nabla_{21}f(x, y^*(x)) \\
&= G(x, y^*(x)).
\end{aligned} \quad (35)$$

Moreover, we have that

$$\begin{aligned}
\|\nabla^2\Phi(x') - \nabla^2\Phi(x)\| &= \|G(x', y^*(x')) - G(x, y^*(x))\| \\
&\leq L_G[\|x' - x\| + \|y^*(x') - y^*(x)\|] \\
&\leq L_G(1 + \kappa)\|x' - x\|,
\end{aligned} \quad (36)$$

where the last step uses the item 1 of Proposition 1. This proves the item 2.  $\square$

## C Proof of Proposition 3

**Proposition 3** (Potential decrease). *Let Assumption 1 hold. For any  $\alpha, \beta > 0$ , choose  $\epsilon' \leq \frac{\alpha L_1}{\beta L_G}$ ,  $\eta_x \leq (9L_\Phi + 18\alpha + 28\beta)^{-1}$  and  $\eta_y = \frac{2}{L+\mu}$ . Define the potential function  $H_t := \Phi(x_t) + (L_\Phi + 2\alpha + 3\beta)\|s_t\|^3$ . Then, when  $N_t \geq \mathcal{O}(\kappa \ln \frac{L_1\alpha\|s_{t-1}\| + L_1(\alpha + L_2\kappa)\|s_t\|}{L_G\beta\epsilon'^2})$ , the output of Cubic-GDA satisfy the following potential decrease property.*

$$H_{t+1} - H_t \leq -(L_\Phi + \alpha + \beta)(\|s_{t+1}\|^3 + \|s_t\|^3). \quad (2)$$

644 *Proof.* The required number of inner gradient ascent steps is shown below

$$\begin{aligned}
N_0 &\geq \kappa \ln (L_1 \|y_0 - y^*(x_0)\| / (2\beta\epsilon'^2)) \\
N_t &\geq \kappa \ln \left( \frac{2L_1\alpha\|s_{t-1}\| + L_1(\alpha + L_G\kappa)\|s_t\|}{L_G\beta\epsilon'^2} \right) \\
&= \mathcal{O} \left( \kappa \ln \frac{L_1\alpha\|s_{t-1}\| + L_1(\alpha + L_2\kappa)\|s_t\|}{L_G\beta\epsilon'^2} \right); 1 \leq t \leq T'.
\end{aligned} \tag{37}$$

645 To prove eq. (2), we first prove by induction that for any  $t \geq 0$ .

$$\|y_{t+1} - y^*(x_t)\| \leq \frac{\alpha(\|s_t\| + \epsilon')}{L_G} \wedge \frac{\beta(\|s_t\|^2 + \epsilon'^2)}{L_1}; 0 \leq t \leq T' - 1. \tag{38}$$

646 Note that  $y_{t+1}$  is obtained by applying  $N_t$  gradient ascent steps starting from  $y_t$ . Hence, by the  
647 convergence rate of gradient ascent algorithm under strong concavity, we conclude that with learning  
648 rate  $\eta_y = \frac{2}{L+\mu}$ ,

$$\|y_{t+1} - y^*(x_t)\| \leq (1 - \kappa^{-1})^{N_t} \|y_t - y^*(x_t)\|. \tag{39}$$

649 When  $t = 0$ , eq. (39) implies that

$$\begin{aligned}
\|y_1 - y^*(x_0)\| &\leq \|y_0 - y^*(x_0)\| \exp(N_0 \ln(1 - \kappa^{-1})) \\
&\stackrel{(i)}{\leq} \|y_0 - y^*(x_0)\| \exp \left( -\ln \left( \frac{L_1\|y_0 - y^*(x_0)\|}{2\beta\epsilon'^2} \right) \right) \\
&= \frac{2\beta\epsilon'^2}{L_1} \stackrel{(ii)}{\leq} \frac{\alpha(\|s_0\| + \epsilon')}{L_G} \wedge \frac{\beta(\|s_0\|^2 + \epsilon'^2)}{L_1}
\end{aligned} \tag{40}$$

650 where (i) uses eq. (37) and  $\ln(1 - x) \leq -x < 0$  for  $x = \kappa^{-1} \in (0, 1)$  and (ii) uses  $\|s_0\| = \epsilon' \leq \frac{\alpha L_1}{\beta L_G}$ .  
651 Hence, eq. (38) holds when  $t = 0$ .

652 If eq. (38) holds for  $t = k - 1 \in [0, T' - 2]$ , then

$$\begin{aligned}
&\|y_{k+1} - y^*(x_k)\| \\
&\leq (1 - \kappa^{-1})^{N_k} \|y_k - y^*(x_{k-1})\| + (1 - \kappa^{-1})^{N_k} \|y^*(x_{k-1}) - y^*(x_k)\| \\
&\stackrel{(i)}{\leq} \exp(N_k \ln(1 - \kappa^{-1})) \left( \left( \frac{\alpha(\|s_{k-1}\| + \epsilon')}{L_G} \wedge \frac{\beta(\|s_{k-1}\|^2 + \epsilon'^2)}{L_1} \right) + \kappa\|s_k\| \right) \\
&\stackrel{(ii)}{\leq} \exp \left( -\ln \left( \frac{2L_1\alpha\|s_{k-1}\| + L_1(\alpha + L_G\kappa)\|s_k\|}{L_G\beta\epsilon'^2} \right) \right) \left( \frac{\alpha(\|s_{k-1}\| + \epsilon')}{L_G} + \kappa\|s_k\| \right) \\
&\stackrel{(iii)}{\leq} \frac{L_G\beta\epsilon'^2}{2L_1\alpha\|s_{k-1}\| + L_1(\alpha + L_G\kappa)\|s_k\|} \frac{\alpha(2\|s_{k-1}\| + \|s_k\|) + L_G\kappa\|s_k\|}{L_G} \\
&= \frac{\beta\epsilon'^2}{L_1} \stackrel{(iv)}{=} \frac{\alpha\epsilon'}{L_G} \wedge \frac{\beta\epsilon'^2}{L_1} \leq \frac{\alpha(\|s_k\| + \epsilon')}{L_G} \wedge \frac{\beta(\|s_k\|^2 + \epsilon'^2)}{L_1}
\end{aligned}$$

653 where (i) uses eq. (38) for  $t = k - 1$  and the fact that  $y^*$  is  $\kappa$ -Lipschitz mapping (see [Lin et al., 2020,  
654 Chen et al., 2021] for the proof), (ii) uses  $\ln(1 - \kappa^{-1}) \leq -\kappa^{-1}$  and eq. (37), (iii) uses  $\epsilon' \leq$   
655  $\|s_{k-1}\| \vee \|s_k\| \leq \|s_{k-1}\| + \|s_k\|$  for  $k \leq T' - 1$ , and (iv) uses the condition that  $\epsilon' \leq \frac{\alpha L_1}{\beta L_G}$ . This  
656 proves eq. (38) holds for  $t = k$  and thus for all  $t \in [0, T' - 1]$ , which further implies eqs. (22) &  
657 (23). Hence, by Lemma 4, we prove that eq. (2) holds for all  $0 \leq t \leq T' - 1$ .  $\square$

## 658 D Proof of Theorem 1

659 **Theorem 1** (Global convergence rate). *Let the conditions of Proposition 3 hold with  $\alpha = \beta = L_\Phi$ .  
660 For any  $0 < \epsilon \leq \frac{L_1\sqrt{33}L_\Phi}{L_G}$ , choose  $\epsilon' = \frac{\epsilon}{\sqrt{33}L_\Phi}$  and  $T \geq \frac{\Phi(x_0) - \Phi^* + 8L_\Phi\epsilon'^2}{3L_\Phi\epsilon'^3}$ . Then, the output of  
661 Cubic-GDA satisfies:*

$$\mu(x_{T'}) \leq \epsilon. \tag{5}$$

662 Consequently, the total number of cubic iterations satisfies  $T' \leq \mathcal{O}(\sqrt{L_2}\kappa^{1.5}\epsilon^{-3})$ , and the total  
663 number of gradient ascent iterations satisfies  $\sum_{t=0}^{T'-1} N_t \leq \tilde{\mathcal{O}}(\sqrt{L_2}\kappa^{2.5}\epsilon^{-3})$ .

664 *Proof.* Substituting  $\alpha = \beta = L_\Phi = L_2(1 + \kappa)^3$  and  $\epsilon' = \frac{\epsilon}{\sqrt{33L_\Phi}}$  into Lemma 5 yields that when  
 665  $T \geq \sqrt{33L_\Phi} \frac{33(\Phi(x_0) - \Phi^*) + 8\epsilon^2}{3\epsilon^3}$  and  $\eta_x = (55L_\Phi)^{-1}$ , we have  $T' \leq \sqrt{33L_\Phi} \frac{33(\Phi(x_0) - \Phi^*) + 8\epsilon^2}{3\epsilon^3} =$   
 666  $\mathcal{O}(\sqrt{L_2}\kappa^{1.5}\epsilon^{-3}) \leq T$ , and moreover,

$$\begin{aligned} \|\nabla\Phi(x_{T'})\| &\leq \left(\frac{1}{2\eta_x} + L_\Phi + 2\alpha + 2\beta\right)\epsilon'^2 \leq \epsilon^2, \\ \lambda_{\min}(\nabla^2\Phi(x_{T'})) &\geq -\left(\frac{1}{2\eta_x} + L_\Phi + 2\alpha\right)\epsilon' \geq -\sqrt{33L_\Phi}\epsilon. \end{aligned}$$

667 This proves eq. (5).

668 Note that the number of gradient ascent iterations  $N_t$  should satisfy eq. (37). Substituting  $\alpha = \beta =$   
 669  $L_\Phi = L_2(1 + \kappa)^3$  and  $\epsilon' = \frac{\epsilon}{\sqrt{33L_\Phi}}$  into eq. (37) yields that

$$\begin{aligned} N_0 &\geq \kappa \ln(L_1\|y_0 - y^*(x_0)\|/(2\beta\epsilon'^2)) = \kappa \ln(33L_1\|y_0 - y^*(x_0)\|/(2\epsilon^2)) \\ N_t &\geq \kappa \ln\left(\frac{2L_1\alpha\|s_{t-1}\| + L_1(\alpha + L_G\kappa)\|s_t\|}{L_G\beta\epsilon'^2}\right) \\ &\stackrel{(i)}{=} \kappa \ln\left(\frac{66L_1(1 + \kappa)\|s_{t-1}\| + 33L_1(2 + \kappa)\|s_t\|}{\epsilon^2}\right); 1 \leq t \leq T' \end{aligned}$$

670 where (i) uses  $L_G = L_2(1 + \kappa)^2$  and  $L_\Phi = L_2(1 + \kappa)^3$  in Proposition 2.

671 When we select  $N_t$  such that the above holds with equality, then the total number of gradient ascent  
 672 iterations is upper bounded as follows

$$\begin{aligned} \sum_{t=0}^{T'-1} N_t &= \kappa \ln(33L_1\|y_0 - y^*(x_0)\|/(2\epsilon^2)) + \kappa \sum_{t=0}^{T'-1} \ln\left(\frac{66L_1(1 + \kappa)\|s_{t-1}\| + 33L_1(2 + \kappa)\|s_t\|}{\epsilon^2}\right) \\ &\leq \kappa \ln(33L_1\|y_0 - y^*(x_0)\|/(2\epsilon^2)) + \kappa \sum_{t=0}^{T'-1} \ln(\|s_{t-1}\| + \|s_t\|) + \kappa T' \ln(66L_1\epsilon^{-2}(1 + \kappa)) \\ &\stackrel{(i)}{\leq} \kappa \ln(33L_1\|y_0 - y^*(x_0)\|/(2\epsilon^2)) + \frac{\kappa T'}{3} \frac{1}{T'} \sum_{t=0}^{T'-1} \ln(4\|s_{t-1}\|^3 + 4\|s_t\|^3) \\ &\quad + \kappa T' \ln(66L_1\epsilon^{-2}(1 + \kappa)) \\ &\stackrel{(ii)}{\leq} \kappa \ln(33L_1\|y_0 - y^*(x_0)\|/(2\epsilon^2)) + \frac{\kappa T'}{3} \ln\left(\frac{4}{T'} \sum_{t=0}^{T'-1} (\|s_{t-1}\|^3 + \|s_t\|^3)\right) \\ &\quad + \kappa T' \ln(66L_1\epsilon^{-2}(1 + \kappa)) \\ &\stackrel{(iii)}{\leq} \kappa \ln(33L_1\|y_0 - y^*(x_0)\|/(2\epsilon^2)) + \frac{\kappa T'}{3} \ln\left(\frac{4(H_0 - H^*)}{3L_\Phi T'}\right) \\ &\quad + \kappa T' \ln(66L_1\epsilon^{-2}(1 + \kappa)) \\ &= \tilde{\mathcal{O}}(\kappa T') \leq \tilde{\mathcal{O}}(\sqrt{L_2}\kappa^{2.5}\epsilon^{-3}) \end{aligned} \tag{41}$$

673 where (i) uses  $(a + b)^3 \leq 4(a^3 + b^3)$  for any  $a, b \geq 0$ , (ii) applies Jensen's inequality to the concave  
 674 function  $\ln(\cdot)$ , and (iii) telescopes eq. (2) over  $t = 0, 1, \dots, T' - 1$ .  $\square$

## 675 E Proof of Theorem 2

676 **Theorem 2** (Convergence and sample complexity). *Let Assumption 2 and Theorem 3 hold. For*  
 677  $0 < \epsilon \leq \frac{L_1\sqrt{33L_\Phi}}{L_G}$ , *choose*  $\epsilon' = \frac{\epsilon}{\sqrt{33L_\Phi}}$ ,  $\eta_x \leq \frac{1}{55L_\Phi}$ ,  $T \geq \frac{\Phi(x_0) - \Phi^* + 8L_\Phi\epsilon'^2}{3L_\Phi\epsilon'^3}$  *and*  $N_t \geq$   
 678  $\mathcal{O}\left(\frac{L_0 \ln(1/\delta) + L_0^2}{\kappa^{-2}(L_\Phi^2\|s_t\|^4 + \epsilon^4) \wedge L_\Phi^2(\|s_t\|^2 + \epsilon^2/L_\Phi)}\right)$ . *Moreover, in iteration  $t$ , choose the batch sizes according to*  
 679 *eqs. (8) and (9) with the inexactness given by*

$$\epsilon_1(t) = \frac{L_\Phi}{2} \left( \|s_t\|^2 + \frac{\epsilon^2}{33L_\Phi} \right) \wedge 2L_0, \quad \epsilon_2(t) = \frac{L_\Phi}{2(\kappa + 1)^2} \left( \|s_t\| + \frac{\epsilon}{\sqrt{33L_\Phi}} \right) \wedge 4L_1.$$

680 Then, the output of Stochastic Cubic-GDA satisfies

$$\mu(x_{T'}) \leq \epsilon. \quad (13)$$

681 Consequently, the total number of cubic iterations satisfies  $T' \leq \mathcal{O}(\sqrt{L_2} \kappa^{1.5} \epsilon^{-3})$ , the total number  
 682 of queried gradient samples satisfies  $\sum_{t'=0}^{T'} (N_t + |B_1(t)|) \leq \mathcal{O}\left(\frac{L_0^2 \kappa^{3.5} \sqrt{L_2}}{\epsilon^7} \ln \frac{m}{\delta}\right)$ , and the total  
 683 number of queried Jacobian samples satisfies  $\sum_{t=0}^{T'-1} \sum_{k=1}^2 \sum_{\ell=1}^2 |B_{k,\ell}(t)| \leq \mathcal{O}\left(\frac{L_1^2 \kappa^{2.5}}{\sqrt{L_2} \epsilon^5} \ln \frac{m+n}{\delta}\right)$ .

684 *Proof.* In Lemma 1, replace  $x, y$  with  $x_t, y_t$ ,  $B_1$  with  $B_1(t)$ , and  $B_{k,\ell}$  with  $B_{k,\ell}(t)$  for any  $k, \ell \in$   
 685  $\{1, 2\}$ , and substitute the following hyperparameters.

$$\begin{aligned} \epsilon_1(t) &= \frac{L_\Phi}{2} \left( \|s_t\|^2 + \frac{\epsilon^2}{33L_\Phi} \right) \wedge 2L_0 = \mathcal{O}(L_\Phi \|s_t\|^2 + \epsilon^2), \\ \epsilon_2(t) &= \frac{L_\Phi}{2(\kappa+1)^2} \left( \|s_t\| + \frac{\epsilon}{\sqrt{33L_\Phi}} \right) \wedge 4L_1 = \mathcal{O}(\kappa^{-2}(L_\Phi \|s_t\| + \sqrt{L_\Phi} \epsilon)). \end{aligned}$$

686 Then, we obtain that using the following batchsizes

$$\begin{cases} |B_1(t)| \geq \mathcal{O}\left(\frac{L_0^2}{(L_\Phi^2 \|s_t\|^4 + \epsilon^4)} \ln \frac{m}{\delta}\right) \\ |B_{k,\ell}(t)| \geq \mathcal{O}\left(\frac{L_1^2 \kappa^4}{L_\Phi (L_\Phi \|s_t\|^2 + \epsilon^2)} \ln \frac{m+n}{\delta}\right) \end{cases}, \quad (42)$$

687 the stochastic approximators satisfy the following error bounds with probability at least  $1 - \delta$ .

$$\|\widehat{\nabla}_1 f(x_t, y_t) - \nabla_1 f(x_t, y_t)\| \leq \epsilon_1(t) \leq \frac{L_\Phi}{2} \left( \|s_t\|^2 + \frac{\epsilon^2}{33L_\Phi} \right), \quad (43)$$

$$\|\widehat{G}(x_t, y_t) - G(x_t, y_t)\| \leq \epsilon_2(t) \leq \frac{L_\Phi}{2} \left( \|s_t\| + \frac{\epsilon}{\sqrt{33L_\Phi}} \right). \quad (44)$$

688 Based on Theorem 3, using the following number of stochastic gradient ascent steps

$$\begin{aligned} N_t &\geq \mathcal{O}\left(\frac{L_0 \ln(1/\delta) + L_0^2}{\mu^2 L_\Phi^2 ((\|s_t\|^2 + \epsilon^2/(33L_\Phi))/L_1) \wedge ((\|s_t\| + \epsilon/\sqrt{33L_\Phi})/L_G))^2}\right) \\ &\stackrel{(i)}{=} \mathcal{O}\left(\frac{L_0 \ln(1/\delta) + L_0^2}{((L_\Phi \|s_t\|^2 + \epsilon^2)/\kappa) \wedge L_1 (\|s_t\| + \epsilon/\sqrt{L_\Phi})^2}\right) \\ &= \mathcal{O}\left(\frac{L_0 \ln(1/\delta) + L_0^2}{\kappa^{-2}(L_\Phi^2 \|s_t\|^4 + \epsilon^4) \wedge L_1^2 (\|s_t\|^2 + \epsilon^2/L_\Phi)}\right), \end{aligned} \quad (45)$$

689 where (i) uses  $\kappa = L_1/\mu$  and  $L_\Phi = L_G(1 + \kappa)$  (Proposition 2). we have

$$\begin{aligned} \|y_{t+1} - y^*(x_t)\| &\leq \mathcal{O}\left(\sqrt{\frac{L_0 \ln(1/\delta) + L_0^2}{\mu^2 N_t}}\right) \\ &\leq \frac{L_\Phi}{2} \min\left(\frac{1}{L_1} \left(\|s_t\|^2 + \frac{\epsilon^2}{33L_\Phi}\right), \frac{1}{L_G} \left(\|s_t\| + \frac{\epsilon}{\sqrt{33L_\Phi}}\right)\right). \end{aligned} \quad (46)$$

690 Therefore,

$$\begin{aligned} &\|\nabla \Phi(x_t) - \widehat{\nabla}_1 f(x_t, y_{t+1})\| \\ &\stackrel{(i)}{\leq} \|\nabla_1 f(x_t, y^*(x_t)) - \nabla_1 f(x_t, y_{t+1})\| + \|\widehat{\nabla}_1 f(x_t, y_{t+1}) - \nabla_1 f(x_t, y_{t+1})\| \\ &\stackrel{(ii)}{\leq} L_1 \|y_{t+1} - y^*(x_t)\| + \frac{L_\Phi}{2} \left( \|s_t\|^2 + \frac{\epsilon^2}{33L_\Phi} \right) \\ &\stackrel{(iii)}{\leq} L_\Phi \left( \|s_t\|^2 + \frac{\epsilon^2}{33L_\Phi} \right), \end{aligned} \quad (47)$$



where (i) uses  $\nabla\Phi(x) = \nabla_1 f(x, y^*(x))$  in Proposition 1, (ii) uses eq. (43) and Assumption 1, and (iii) uses eq. (46).

$$\begin{aligned}
& \|\nabla^2\Phi(x_t) - \widehat{G}(x_t, y_{t+1})\| \\
& \stackrel{(i)}{\leq} \|G(x_t, y^*(x_t)) - G(x_t, y_{t+1})\| + \|\widehat{G}(x_t, y_{t+1}) - G(x_t, y_{t+1})\| \\
& \stackrel{(ii)}{\leq} L_G \|y_{t+1} - y^*(x_t)\| + \frac{L_\Phi}{2} \left( \|s_t\| + \frac{\epsilon}{\sqrt{33L_\Phi}} \right) \\
& \stackrel{(iii)}{\leq} L_\Phi \left( \|s_t\| + \frac{\epsilon}{\sqrt{33L_\Phi}} \right), \tag{48}
\end{aligned}$$

where (i) uses  $\nabla^2\Phi(x) = G(x, y^*(x))$  in Proposition 2, (ii) uses eq. (44) and the item 1 of Proposition 2, and (iii) uses eq. (46). Eqs. (47) & (48) imply that the conditions (22) & (23) hold with  $\alpha = \beta = L_\Phi = L_2(1 + \kappa)^3$  and  $\epsilon' = \frac{\epsilon}{\sqrt{33L_\Phi}}$ . In Lemma 5, by substituting these values of  $\alpha$ ,  $\beta$ ,  $\epsilon'$  and  $\eta_x = (55L_\Phi)^{-1}$ , we obtain that when  $T \geq \frac{\Phi(x_0) - \Phi^* + 8L_\Phi\epsilon'^2}{3L_\Phi\epsilon'^3}$ , we have  $T' \leq \sqrt{33L_\Phi} \frac{33(\Phi(x_0) - \Phi^*) + 8\epsilon^2}{3\epsilon^3} = \mathcal{O}(\sqrt{L_2}\kappa^{1.5}\epsilon^{-3}) \leq T$ , and moreover,

$$\begin{aligned}
\|\nabla\Phi(x_{T'})\| & \leq \left( \frac{1}{2\eta_x} + L_\Phi + 2\alpha + 2\beta \right) \epsilon'^2 \leq \epsilon^2, \\
\lambda_{\min}(\nabla^2\Phi(x_{T'})) & \geq -\left( \frac{1}{2\eta_x} + L_\Phi + 2\alpha \right) \epsilon' \stackrel{(i)}{\geq} -\sqrt{33L_\Phi}\epsilon,
\end{aligned}$$

This proves that eq. (13) holds with probability at least  $1 - \delta$ .

Choosing both  $N_t$  in eq. (45) and the batchsizes in eq. (42) with equality, the number of gradient computations has the following upper bound.

$$\begin{aligned}
& \sum_{t=0}^{T'-1} (N_t + |B_1(t)|) \\
& = \sum_{t=0}^{T'-1} \mathcal{O}\left( \frac{L_0 \ln(1/\delta) + L_0^2}{\kappa^{-2}(L_\Phi^2 \|s_t\|^4 + \epsilon^4) \wedge L_1^2(\|s_t\|^2 + \epsilon^2/L_\Phi)} + \frac{L_0^2}{L_\Phi^2 \|s_t\|^4 + \epsilon^4} \ln \frac{m}{\delta} \right) \\
& \leq \sum_{t=0}^{T'-1} \mathcal{O}\left( \frac{L_0 \ln(1/\delta) + L_0^2}{\epsilon^4 \kappa^{-2} \wedge L_1^2 \epsilon^2 / L_\Phi} + \frac{L_0^2}{\epsilon^4} \ln \frac{m}{\delta} \right) \\
& \stackrel{(i)}{\leq} T' \mathcal{O}\left( \frac{L_0 \kappa^2}{\epsilon^4} (\ln(1/\delta) + L_0) + \frac{L_0^2}{\epsilon^4} \ln \frac{m}{\delta} \right) \\
& \stackrel{(ii)}{\leq} \mathcal{O}(\sqrt{L_2}\kappa^{1.5}\epsilon^{-3}) \mathcal{O}\left( \frac{L_0^2 \kappa^2}{\epsilon^4} \ln \frac{m}{\delta} \right) \\
& \leq \mathcal{O}\left( \frac{L_0^2 \kappa^{3.5} \sqrt{L_2}}{\epsilon^7} \ln \frac{m}{\delta} \right) \tag{49}
\end{aligned}$$

where (i) uses  $\epsilon' = \frac{\epsilon}{\sqrt{33L_\Phi}} \leq \frac{L_1}{L_G} = \frac{L_1(1+\kappa)}{L_\Phi}$  which implies that  $\epsilon^4 \kappa^{-2} \leq \mathcal{O}(L_1^2 \epsilon^2 / L_\Phi)$ , (ii) uses  $T' \leq \mathcal{O}(\sqrt{L_2}\kappa^{1.5}\epsilon^{-3})$  we proved above. The number of Hessian computations has the following upper bound.

$$\begin{aligned}
& \sum_{t=0}^{T'-1} \sum_{k=1}^2 \sum_{\ell=1}^2 |B_{k,\ell}(t)| \\
& = \sum_{t=0}^{T'-1} \mathcal{O}\left( \frac{L_1^2 \kappa^4}{L_\Phi (L_\Phi \|s_t\|^2 + \epsilon^2)} \ln \frac{m+n}{\delta} \right) \\
& \leq \sum_{t=0}^{T'-1} \mathcal{O}\left( \frac{L_1^2 \kappa^4}{L_\Phi \epsilon^2} \ln \frac{m+n}{\delta} \right)
\end{aligned}$$

$$\begin{aligned}
&\stackrel{(i)}{\leq} T' \mathcal{O}\left(\frac{L_1^2 \kappa}{L_2 \epsilon^2} \ln \frac{m+n}{\delta}\right) \\
&\stackrel{(ii)}{\leq} \mathcal{O}\left(\frac{L_1^2 \kappa^{2.5}}{\sqrt{L_2} \epsilon^5} \ln \frac{m+n}{\delta}\right)
\end{aligned} \tag{50}$$

704 where (i) uses  $L_\Phi = L_2(1 + \kappa)^3 = \mathcal{O}(L_2 \kappa^3)$ , (ii) uses  $T' \leq \sqrt{33L_\Phi} \frac{33(\Phi(x_0) - \Phi^*) + 8\epsilon^2}{3\epsilon^3} =$   
705  $\mathcal{O}(\sqrt{L_2} \kappa^{1.5} \epsilon^{-3})$  we proved above.  $\square$

## 706 F Convergence Rate of SGA

707 The following high-probability convergence rate of SGA is a direct application of the Theorem 3.1 of  
708 [Harvey et al., 2019].

709 **Theorem 3.** *Let Assumption 2 hold. For all  $t, k$ , assume that  $\|\nabla_2 f(x_t, \tilde{y}_k)\| \leq L_0$  and  
710  $\|\widehat{\nabla}_2 f(x_t, \tilde{y}_k) - \nabla_2 f(x_t, \tilde{y}_k)\| \leq 1$  almost surely. The inner stochastic gradient ascent steps in  
711 Algorithm 2 converges at the following rate with probability at least  $1 - \delta$ .*

$$\|y_{t+1} - y^*(x_t)\| \leq \mathcal{O}\left(\sqrt{\frac{L_0 \ln(1/\delta) + L_0^2}{\mu^2 N_t}}\right).$$

712 *Proof.* Based on Theorem 3.1 of [Harvey et al., 2019], the inner SGA steps in Algorithm 2 has the  
713 following convergence rate with probability at least  $1 - \delta$ .

$$f(x_t, y^*(x_t)) - f(x_t, y_{t+1}) \leq \mathcal{O}\left(\frac{L_0 \ln(1/\delta) + L_0^2}{\mu N_t}\right), \tag{51}$$

714 which by  $\mu$ -strong concavity of  $f(x_t, \cdot)$  proves the following convergence rate.

$$\|y_{t+1} - y^*(x_t)\| \leq \sqrt{2(f(x_t, y^*(x_t)) - f(x_t, y_{t+1})) / \mu} \leq \mathcal{O}\left(\sqrt{\frac{L_0 \ln(1/\delta) + L_0^2}{\mu^2 N_t}}\right).$$

715  $\square$

## 716 G Compute Jacobian-Vector Product

717 In Algorithm 1 (and similarly for Algorithm 2), the key step is the cubic regularization update, which  
718 requires solving the following generic cubic sub-problem.

$$\begin{aligned}
&\underset{s}{\operatorname{argmin}} \nabla_1 f(x, y)^\top s + \frac{1}{2} s^\top G(x, y) s + \frac{1}{6\eta_x} \|s\|^3, \\
&\text{where } G(x, y) = [\nabla_{11} f - \nabla_{12} f (\nabla_{22} f)^{-1} \nabla_{21} f](x, y).
\end{aligned}$$

719 In the literature, many gradient-based cubic-solvers have been developed to efficiently solve cubic  
720 sub-problems, and their convergence guarantee and computation complexity are well established  
721 [Carmon and Duchi, 2016, Tripuraneni et al., 2018]. In particular, when implementing these cubic-  
722 solvers to solve the above cubic sub-problem, one needs to query the Hessian-vector product  $G(x, y) \cdot u$   
723 for a general vector  $u$ . This quantity can be efficiently computed as we elaborate below.

724 First, note that for any vector  $v$ , the Jacobian-vector products  $\nabla_{k\ell} f(x, y) \cdot v$  for all  $k, \ell \in \{1, 2\}$  can  
725 be computed via standard auto-differentiation as follows

$$\nabla_{k\ell} f(x, y) \cdot v = \nabla_\ell (\nabla_k f(x, y)^\top v), \quad \forall k, \ell \in \{1, 2\}.$$

726 Therefore, we can query the above Jacobian-vector product oracle to compute

$$z_1 := \nabla_{11} f(x, y) \cdot u, \quad z_2 := \nabla_{21} f(x, y) \cdot u.$$

727 Then, we have  $G(x, y) \cdot u = z_1 - [\nabla_{12} f (\nabla_{22} f)^{-1}](x, y) \cdot z_2$ . Note that the quantity  $z_3 :=$   
728  $(\nabla_{22} f(x, y))^{-1} \cdot z_2$  can be computed by solving the linear system

$$\nabla_{22} f(x, y) \cdot z_3 = z_2$$

729 using standard conjugate gradient solvers. Lastly, we query another Jacobian-vector product oracle to  
730 compute

$$z_4 := \nabla_{12} f(x, y) \cdot z_3.$$

731 Finally, the Hessian-vector product can be computed as  $G(x, y) \cdot u = z_1 - z_4$ .

732
